# Supplementary material for: Automated rock joint trace mapping using a supervised learning model trained on synthetic data generated by parametric modelling
Source: arXiv:2602.07590 ancillary file (2026-02-07)
Supplement: Supplementary file 1 [file Appendix_A_Parametric_modelling_DFN_dataset.pdf]

# A Parametric modelling of the synthetic discrete fracture network dataset and associated results

This appendix provides detailed methodological descriptions, software-specific implementations, and auxiliary analyses that support the methods presented in the main text.

We use the proprietary software FracMan (version 8.30) to generate a grown fracture network that consists of three joint sets and random joints. To enhance the generalisability of the synthetic Discrete Fracture Network (DFN) dataset, we perform a parametric study to select 27 block shapes that scatter over two commonly used rock block shape classifications by Palmström (1995) and Singh et al. (2022). For each of these 27 primary block shapes, we configure a unique set of input fracture parameters for generating a DFN in FracMan. For each DFN, we apply eight different rock texture from Poly Haven, a free 3D asset library, for generating rendered rock mass images with different textures, simulating different rock types. The workflow for generating the synthetic DFN dataset is illustrated in Fig. 4 as seven steps. Details for each step in the workflow will be described below.

We develop a Grasshopper script to carry out a parametric study for getting different block shapes across commonly used rock block shape classifications (Step 1). Grasshopper is a visual programming language and environment within the Rhinoceros 3D (Rhino) computer-aided design application. In the parametric study, we create parallelepipeds (hexahedrons with three pairs of parallel faces) first by varying the relative length of a box with a constant volume of 5 $m^3$ along its $x$-, $y$- , and $z$-directions, then by rotating each parallel face pair of the box with at various degrees (-30°, -15°, 0°, 15°, and 30°) around each face's $x$-, $y$- , and $z$-axes. This contributes to a total of 12 variables (parameters). Using a Grasshopper-plug-in, Tunny (Natsume, 2024), we perform a quasi Monte-Carlo analysis to obtain 8192 combinations of the 12 variables across its value intervals. The block shape parameters for the 8192 parallelepipeds are determined using the classification systems by Palmström (1995) and Singh et al. (2022). Based on the results of the calculated block shape parameters (Fig. 3), we select 27 of the parallelepipeds that represent all the block shape classes and in-between.

In step 2, assuming each of the 27 parallelepipeds to be the predominant block shape of a DFN and bounded by three joint sets, we determine the orientation (dip and dip direction) and the volumetric joint intensity parameter, $P_{32}$ (total joint area per unit volume), for each set of parallel face pairs. The joint orientation and $P_{32}$ are directly used as input parameters for the 'growth' fracture network (Libby et al., 2019) process in FracMan. To determine $P_{32}$, we define a cubic box with a certain edge length as the unit volume and extrapolate each parallelepiped face beyond the cubic box at fixed spacings defined by the shape and volume of the parallelepiped. Consistent with the observations by Taboni et al. (2025) that $P_{32}$ is influenced by the edge length of the boundary of the DFN, $P_{32}$ of all our 27 cases converges at large edge lengths. $P_{32}$ is calculated as the average value determined with edge lengths from 40 m to 100 m. Assuming a chronology of the joint sets, the joint set with the largest $P_{32}$ is the oldest, and vice versa. In FracMan, we assume joints to always terminate

against the other joints in the same set, but with 80% probability against an older set. We implement variability and randomness in the DFN by assuming a Fisher distribution with a concentration constant of 20 for all joint sets' joint orientations. Fracture lengths of the joint set with the largest input $P_{32}$ follow an exponential distribution with a mean and standard deviation at 30 m, whereas those of the other joint sets follow a log-normal distribution (mean = 5 m, standard deviation = 0.5 m, truncated at 0.25 and 15 m, after (Li and Elmo, 2024)). Each DFN is intersected by random joints, which are specified as a joint set in FracMan with fracture lengths distributed exponentially (mean = standard deviation = 30 m) but fully random joint orientation (Fisher distribution's concentration constant equals zero). Random joints will not terminate against any other joints.

The 3D planar fracture polygons are exported in FAB format from FracMan and then converted to STL format using proprietary software DFN.lab (Fractory, 2022). The converted STL files will be compatible for further analysis. We implement three processes to get more realistic 3D rock mass models that simulate blasted rock cuts. First, using the two-bench slope model, we use proprietary software Rocscience RocSlope3 to compute blocks and kinematic analyses on the computed blocks for each DFN (Step 3). A joint friction angle of 20° and zero cohesion is assumed using the Mohr-Coulomb strength criterion for all the joints. After the kinematic analysis, we export a socketed slope surface by removing failed blocks. The removal of failed blocks is to simulate a newly-blasted slope with a natural fallout of unstable blocks and eventually after machine/manual scaling. Secondly, we use the Grasshopper plug-in 4D Noise (Piacentino, 2011) to apply a Perlin noise function (Perlin and Hoffert, 1989) with a scaling coefficient of 0.2 on 1000 randomly populated 3D points over the socketed slope surfaces (Step 4). The final slope surfaces are slightly rough like real rock slope surfaces but still depict their two-bench geometry. Finally, we generate joint traces by intersecting the DFNs with their corresponding final slope surface via FracMan. Similar to the labels of the real-world rock slope dataset (Section 4.1.2), we apply joint waviness and thickness to the joints in Rhino/Grasshopper (Step 5). However, for the synthetic DFN dataset, we apply these two geometric variables directly to the intersecting joint curves for visualisation in the rock mass and label images.

Note that $T$ is also the absolute visible line width with respect to the model space in Rhino. We set $T_{\min}$ and $T_{\max}$ arbitrarily to 1 mm and 10 cm, respectively.

The rendering of the image (Step 7) follows the procedures described in Section 4.2.1. In all the rendered images, the joint curves are displayed in black. For the rock mass rendered images, we simulate shadows from the edge effect on both sides of the joint opening by multiplying $T$ by 1.5 and applying an alpha value of 100 to display a transparency colour. We let $0 \leq \alpha \leq 255$, where $\alpha = 0$ is fully transparent and $\alpha = 255$ is opaque. We overlay narrower opaque joint curves to represent the opening that may be visible deeper into the rock joint. The narrower curves have the absolute line width of $T \times 0.5$. Since the joint curves are planar, to make the joint traces more realistic, we further simulate the narrower joint curves with a slightly rough profile. The rough joint curve profile is done by redrawing the narrower curves from random points emitted from the joint curves at about 10 cm along the joint curve and within the joint curves' visual radius (i.e. $T/2$). For the label images, we draw the joint traces

using the planar joint curves with visual thickness equals $T$. However, we only display those joint traces with $T \geq 1$ cm, considering very thin joint traces are likely not visible in photos or point clouds.

For texture mapping, we map the diffuse map of each of the Poly Haven texture to the rough socketed slope mesh via the Box mapping function in the Grasshopper plug-in Human (Heumann, 2012) (Step 6). The diffuse map is the albedo map of an image with most of shading removed (Poly Haven, 2025). To ensure a realistic texture in rock mass images to the real-world scale, all the eight different textures are mapped from a 30 × 30 × 30 m box to the slope mesh.

Since rock jointing is directly imported from the generated DFNs, the labels for the dataset are nearly perfect. However, in cases where a joint rock mass image is used as a texture, the joint traces in the background texture will likely result in false positives in the machine learning (ML) predictions.

To characterise the generalisability of the synthetic DFN dataset, we analyse both block shape variability and joint trace network topology. For each of the 27 selected DFNs, we determine the volume and shape parameters for all the valid blocks computed with RocSlope3. The distribution of block shape classes defined by the classification schemes of Palmström (1995) and Singh et al. (2022) are analysed separately. Joint trace networks are obtained using FracMan by intersecting the DFNs with Perlin-noised slope surfaces, and connectivity was quantified using node-type analysis following (Manzocchi, 2002; Sanderson and Nixon, 2015). Intersections were classified into I-nodes (terminations), Y-nodes (abutting intersections), and X-nodes (cross-cutting). I-nodes were only counted if located more than 0.1 m from the slope edge to reduce boundary effects, and Y-nodes were also counted where a fracture terminates before or after another within the same 0.1 m threshold. All geometric and topological metrics were computed using custom Grasshopper scripts.

## References


Fractory (2022) DFN.Lab a complete DFN Software tool. https://fractorylab.org/dfnlab-software/. Accessed 29 December 2025

Heumann A (2012) Human. https://www.food4rhino.com/en/app/human. Accessed 29 December 2025

Li Y, Elmo D (2024) Application of the network connectivity index on fragmentation assessment in cave mine design. In: Cumming-Potvin D, Andrieux P (eds) Deep Mining 2024: Proceedings of the 10th International Conference on Deep and High Stress Mining. Australian Centre for Geomechanics, Perth, pp 1091–1102, https://doi.org/10.36487/ACG_repo/2465_70

Libby S, Hartley L, Turnbull R, et al (2019) Grown Discrete Fracture Networks: a new method for generating fractures according to their deformation history. In: Proceedings of the 53rd US Rock Mechanics/Geomechanics Symposium, pp 23–26

Manzocchi T (2002) The connectivity of two-dimensional networks of spatially correlated fractures. Water Resources Research 38(9):1–1–1–20. https://doi.org/10.1029/2000WR000180

Natsume H (2024) Tunny, The Grasshopper optimization tool. Version 0.12.0. https://github.com/hrntsm/Tunny. Accessed 29 December 2025

Palmström A (1995) RMi-a rock mass characterization system for rock engineering purposes. PhD. thesis. PhD thesis, University of Oslo, Norway

Perlin K, Hoffert EM (1989) Hypertexture. SIGGRAPH Comput Graph 23(3):253–262. https://doi.org/10.1145/74334.74359

Piacentino G (2011) 4D Noise. https://www.food4rhino.com/en/app/4d-noise. Accessed 29 December 2025

Poly Haven (2025) FAQ | Poly Haven Wiki. https://docs.polyhaven.com/en/faq. Accessed 29 December 2025

Sanderson DJ, Nixon CW (2015) The use of topology in fracture network characterization. Journal of Structural Geology 72:55–66. https://doi.org/10.1016/j.jsg.2015.01.005

Singh J, Pradhan SP, Singh M, et al (2022) Modified block shape characterization method for classification of fractured rock: A python-based GUI tool. Computers & Geosciences 164:105125. https://doi.org/10.1016/j.cageo.2022.105125

Taboni B, Ferrero AM, Umili G (2025) Block Volume and Shape: Comparison of Calculation Methods and Investigation of Possible Relationships. Rock Mech Rock Eng 58(1):697–721. https://doi.org/10.1007/s00603-024-04178-w
