# Supplementary material for: Automated rock joint trace mapping using a supervised learning model trained on synthetic data generated by parametric modelling
Source: arXiv:2602.07590 ancillary file (2026-02-07)
Supplement: Supplementary file 2 [file Appendix_B_REFORMS_checklist.pdf]

# Checklist for reporting ML-based science

## (template downloaded 4<sup>th</sup> April 2025)

### Module 1: Study goals

1a. Population or distribution about which the scientific claim is made.

Rock joint traces in rock slopes, both man-made rock cuts and natural rock cliffs.

1b. Motivation for choosing this population or distribution (1a.).

Rock joints are critical to slope stability analysis and support design in infrastructure projects. A fully exposed rock joint on a rock surface consists of both surfaces and traces. Rock joint surfaces can be extracted directly from 3D models, but rock joint traces, which are usually up to mm wide, are not as detectable from 3D models due to low resolutions. They are more traceable in images with higher resolutions.

1c. Motivation for the use of ML methods in the study.

ML enables automated, scalable segmentation of joint traces from images. However, manual labelling of rock joints is subjective and labour-intensive. We propose using synthetic data to compensate for the problem of a lack of good-quality labels for supervised ML. Our study test and validate a parametric procedure for generating image of synthetic rock mass images with perfect ground truth.

### Module 2: Computational reproducibility

2a. Dataset used for training and evaluating the model along with link or DOI to uniquely identify the dataset.

All datasets used for ML training and evaluation (synthetic DFN, synthetic box, real-world box, real-world rock slope), including datasheets, are available on Zenodo

DOI: [10.5281/zenodo.18078781](https://doi.org/10.5281/zenodo.18078781)

2b. Code used to train and evaluate the model and produce the results reported in the paper along with link or DOI to uniquely identify the version of the code used.

All code used for synthetic data generation, ML training, evaluation, and plotting is available in public repositories listed in the Supplementary Materials. Versioned repositories are hosted on GitHub.

Synthetic data generation: [https://github.com/norwegian-geotechnical-institute/synthetic\\_rockmass\\_image\\_generation\\_for\\_ml](https://github.com/norwegian-geotechnical-institute/synthetic_rockmass_image_generation_for_ml)

ML pipelines: [https://github.com/tfha/syntetic\\_rock\\_joint\\_generation\\_for\\_ml](https://github.com/tfha/syntetic_rock_joint_generation_for_ml)

2c. Description of the computing infrastructure used.

- Hardware infrastructure: CPU, GPU, RAM, disk space etc.
- Operating system.
- Software environment: Programming language and version, documentation of all packages used along with versions and dependencies (e.g., through a requirements.txt file).
- An estimate of the time taken to generate the results.

All software environment details and dependencies are included in the Github repository:

[https://github.com/tfha/syntetic\\_rock\\_joint\\_generation\\_for\\_ml](https://github.com/tfha/syntetic_rock_joint_generation_for_ml)

- Hardware infrastructure: Virtual machines via Azure ML. Standard\_NC6s\_v3 series. Six virtual CPUs, 112 GiB memory, one NVIDIA Tesla V100 GPU with 16 GiB RAM. We used two parallel subprocesses for data loading.
- Operating system: Linux-based Azure ML managed environment
- Software environment: Python, package dependencies controlled and documented using Poetry, see the file pyproject.toml. All packages with versions can be found in the file poetry.lock
- An estimate of the time taken to generate the results: Up to 100 epochs per experiment. Wall-clock time per experiment depends on dataset size and strategy. Box-domain experiments took 4.7 to 31.4 min (average 17.0 min) per experiment, whereas slope-domain experiments took 17.3 to 247.2 min (average 59.9 min) per experiment.

2d. README file which contains instructions for generating the results using the provided dataset and code.

Explicitly stated in Supplementary Materials.

2e. Reproduction script to produce all results reported in the paper<sup>1</sup>.

Reproduction is possible by executing the documented ML pipelines in the provided repository. Experiments are parameterised via configuration files and Azure ML experiment definitions rather than a single monolithic script. All stochastic components (data shuffling, weight initialisation, data augmentation, and training procedures) are controlled by fixed random seed values to ensure deterministic and reproducible results across runs.

## Module 3: Data quality

3a. Source(s) of data, separately for the training and evaluation datasets (if applicable), along with the time when the dataset(s) are collected, the source and process of ground-truth annotations, and other data documentation.

All the relevant information for each dataset is described in separate datasheets. Datasheets for all datasets are included in Zenodo (10.5281/zenodo.18078781), following the template by Gebru T, Morgenstern J, Vecchione B, et al (2021) Datasheets for Datasets. DOI: [10.48550/arXiv.1803.09010](https://doi.org/10.48550/arXiv.1803.09010)

3b. Distribution or set from which the dataset is sampled (i.e., the sampling frame).

Synthetic rock slope datasets are generated via parametric modelling. This study proposed a method to generate a generalised dataset based on a diverse jointing configuration (varied joint spacing and joint orientations, derived from a 5 m<sup>3</sup> cube). Three joint sets plus random joints are common in jointed hard rock. Eight different rock mass textures downloaded from PolyHaven are used, aiming at a variety of colour and patterns.

Real-world rock slope datasets are sampled from selected road cuts in Norway representing jointed hard rock slopes. The road cut sections at E18 Larvik and Rv4 Roa-Gran were chosen because more than one expert has conducted and quality-assured the digital rock joint mapping. The two sites have different lithologies, making the datasets more generalised.

The box datasets are based on dimensions comparable to typical rock block sizes (0.14 m<sup>3</sup>). The synthetic box datasets use a simple box configuration of only seven boxes, but they represent all the possible joint trace occurrence scenarios (trace crossing planes, traces overlapping edges). The same rock mass textures for the synthetic box datasets as the synthetic rock mass datasets are

---

<sup>1</sup> Note that this is a high bar for computational reproducibility. It might not be possible to provide such a script—for instance, if the analysis is run on an academic computing cluster, or if the dataset does not allow for programmatic download.

used, making it possible for direct comparisons between the DFN and box approaches on ML training using synthetic datasets.

The real-world box datasets use the same box dimensions as the synthetic box dataset, but with a more complex box configuration of 13 boxes, which expands the dimensions of joint trace occurrences. A cardbox color and stone pattern in the real-world box dataset are used to further to study whether rock-like pattern can influence the results.

3c. Justification for why the dataset is useful for the modeling task at hand.

Synthetic datasets offer perfect labels for high-quality ML training. Real-world datasets represent real scenarios where the model will be deployed. Box datasets enables an alternative validation approach in a controlled environment.

3d. The definition of the outcome variable of the model along with descriptive statistics, if applicable.

*(The outcome variable is also known as the dependent variable, the target variable, the output variable or the predicted variable).*

The outcome variable is binary: pixel classified as ‘joint trace’ (positive, black) or ‘non joint trace’ (negative, white).

3e. Number of samples in the dataset.

Provided in Table 1.

3f. Percentage of missing data, split by class for a categorical outcome variable.

No missing data concern. We validate dataset files before transformations are applied, via basic validation checks on paired image and label files to ensure:

1. Both image and label files exist at the specified paths
2. Both files can be opened as valid images
3. Image dimensions match between each image and its corresponding label

3g. Justification for why the distribution or set from which the dataset is drawn (3b.) is representative of the one about which the scientific claim is being made (1a.).

See Section 5.1. The synthetic dataset mimics geometrical and visual properties of real-world joint network on rock slopes. The connectivity index,  $C_L$ , of the synthetic joint traces is representative

for natural occurrences, rather than a stochastic rock joint network (Fig .5). Fig. 6 describes the distribution of block volume and block geometry class.

Representativeness is supported by quantitative network topology metrics (node-type proportions and connectivity index), block volume and shape distributions, and by embedding geological constraints through DFN modelling. The dataset is intended as a geological prior rather than a direct statistical replica of any specific site.

## Module 4: Data preprocessing

4a. Identification of whether any samples are excluded with a rationale for why they are excluded.

Some rendered images from the synthetic DFN dataset are captured from the side of the slope, showing the backside of the slope surface. Since it will not be possible to capture images from behind the slope surface in reality, these rendered images will not be used for ML.

4b. How impossible or corrupt samples are dealt with.

See 4a.

4c. All transformations of the dataset from its raw form (3a.) to the form used in the model, for instance, treatment of missing data and normalization —preferably through a flow chart.

Since the raw form of label images (mask images) is in RGB, all the label images are transformed to binary images before machine learning. The binarisation step converts pixels less than the threshold (default: 128) to black (value = 0) to represent rock joints and all other pixels to white pixels (255) to represent the background.

The python script used for this preprocessing step is described in README.md in the Github repository: [https://github.com/tfha/syntetic\\_rock\\_joint\\_generation\\_for\\_ml](https://github.com/tfha/syntetic_rock_joint_generation_for_ml)

Data augmentation, including random flips, rotation, random crop, random affine transforms, random perspective, colour jitter, and Gaussian blur are also implemented for ML training.

## Module 5: Modeling

5a. Detailed descriptions of all models trained, including:

- All features used in the model (including any feature selection).  
No feature selection is used explicitly.

- Types of models implemented (e.g., Random Forests, Neural Networks).  
Convolutional neural networks (CNNs) are used. Pre-trained encoder backbones for U-net and DeepLabv3+ model from ImageNet.

Loss function used.

Dice loss function

5b. Justification for the choice of model types implemented.

We use proven CNN architectures, specifically U-net and DeepLabv3+, which have demonstrated strong performance in crack and joint segmentation. This task is closely related to segmenting rock joint traces in rock outcrops. To save time and computational resources, we use open-source pre-trained versions of these networks for transfer learning. This allows us to build on established feature representations and significantly reduce training time.

5c. Method for evaluating the model(s) reported in the paper, including details of train-test splits or cross-validation folds.

Train/validation split ratio: 0.9/0.1. The trained model is tested on unseen real-world data.

5d. Method for selecting the model(s) reported in the paper.

No specific model configuration has been selected. Experiments were carried out to investigate which training strategy (Finetune or SimpleMixed) and the real:synthetic data ratio to achieve good results.

Quantitatively based on evaluation metrics, including IoU (Intersection over Union), Dice Coefficient, precision, and recall.

Qualitatively based on output mask.

5e. For the model(s) reported in the paper, specify details about the hyperparameter tuning:

- Range of hyper-parameters used and a justification for why this range is reasonable.
- Method to select the best hyper-parameter configuration.
- Specification of all hyper-parameters used to generate results reported in the paper.

Hyperparameter tuning is not the scope of the work

5f. Justification that model comparisons are against appropriate baselines.

We compare using models trained with 100% real data or synthetic data as benchmarks.

## Module 6: Data leakage

6a. Justification that pre-processing (Section 4) and modeling (Section 5) steps only use information from the training dataset (and not the test dataset).

Data splitting is done before preprocessing and modelling

6b. Methods to address dependencies or duplicates between the training and test datasets (e.g. different samples from the same patients are kept in the same dataset partition).

The splits are mutually exclusive, with set-based checks ensuring no overlap or duplicates for training. The data leakage check is logged for each experiment.

6c. Justification that each feature or input used in the model is legitimate for the task at hand and does not lead to leakage.

All the input images are real-world or synthetic representation of rock surface or box configurations. The background of the real-world box datasets is removed. The images contain the visual pattern, texture and contrasts that reflect joint traces from a rock-like background, which are the target of segmentation. No metadata or labels are leaked into the model. Data augmentation has only been applied to training data. Therefore, all the features used by the model are legitimate without data leakage.

## Module 7: Metrics and uncertainty

7a. All metrics used to assess and compare model performance (e.g., accuracy, AUROC etc.). Justify that the metric used to select the final model is suitable for the task.

The ML results are evaluated quantitatively based on metrics, including IoU (Intersection over Union), Dice Coefficient, precision, and recall. These are standard metrics used in many previous studies in image segmentation.

IoU is a measure of the overlap between the predicted and true positive pixels and is used to evaluate the model's accuracy in detecting rock joints in the image.

The Dice Coefficient measures the similarity between the predicted and true positive pixels and is sensitive to how well the model captures fine details.

Precision indicates how many of the predicted joint traces are accurate, while recall shows how many of the true joint traces were detected. Balancing these metrics is key for generalising to different rock masses, as some joints may be subtle and easily missed (low recall) or overestimated (low precision).

The prediction mask images are also evaluated qualitatively based on output masks. This allows us to visually inspect the model's performance and identify any potential issues with the model's predictions.

7b. Uncertainty estimates (e.g., confidence intervals, standard deviations), and details of how these are calculated.

No formal uncertainty estimates (e.g., confidence intervals or variance estimates) are reported. Model variability is explored indirectly through multiple experiments across domains, data proportions, and training strategies.

7c. Justification for the choice of statistical tests (if used) and a check for the assumptions of the statistical test.

No formal statistical hypothesis tests were conducted. The study relies on descriptive performance metrics and structured qualitative assessment rather than inferential statistical testing.

## Module 8: Generalizability and limitations

8a. Evidence of external validity.

Demonstrating external validity is the primary objective of this study. The methodology is explicitly designed to test whether machine-learning models trained on parameter-controlled synthetic data can generalise to independent real-world dataset textures from different texture and geometries. External validity is therefore assessed through evaluation on unseen real-world rock slopes (E18 Larvik and Rv4 Roa–Gran) and controlled real-world box experiments.

8b. Contexts in which the authors do not expect the study's findings to hold.

Findings may not hold in heavily jointed or heavily weathered rock, and other rock types that we have not trained or tested. They may not hold in images from tunnels or other dimensions such as rock cores.
